# Supplementary material for: Scratching Visual Transformer's Back with Uniform Attention
Source: arXiv:2210.08457 source file (2024-12-26)
Supplement: Supplementary file 1 [file 00_a_guide.tex]

We present the experiment setup and additional experiments not included in the main paper.
The contents of this appendix are listed as follows:

\section*{Contents}
\textbf{A \ \ \ Details of Experiments Setup\\} \\
\text{\qquad A.1 \ \ \ Datasets} \\ \\
\text{\qquad A.2 \ \ \ Models} \\ \\
\text{\qquad A.3 \ \ \ Hyper-parameters} \\ \\
\textbf{B \ \ \ Additional Experiments\\} \\
\text{\qquad B.1 \ \ \ Training Curve} \\ \\
\text{\qquad B.2 \ \ \ Attention Visualization} \\ \\
\text{\qquad B.3 \ \ \ Other Architectures} \\ \\
\text{\qquad B.4 \ \ \ Robustness of ADE20K} \\ \\
\text{\qquad B.5 \ \ \ Discussion on Position of CB} \\ \\
\text{\qquad B.6 \ \ \ Utilizing The Class Token} \\ \\

\noindent\rule{\linewidth}{0.2pt}
