# Supplementary material for: Scratching Visual Transformer's Back with Uniform Attention
Source: arXiv:2210.08457 source file (2024-12-26)
Supplement: Supplementary file 2 [file vis.tex]

\begin{figure}
    \centering

    \begin{tabular}{c}
        \includegraphics[width=.15\linewidth]{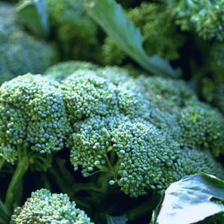}
    \end{tabular} %
    \begin{tabular}{c}
        \includegraphics[width=.75\linewidth]{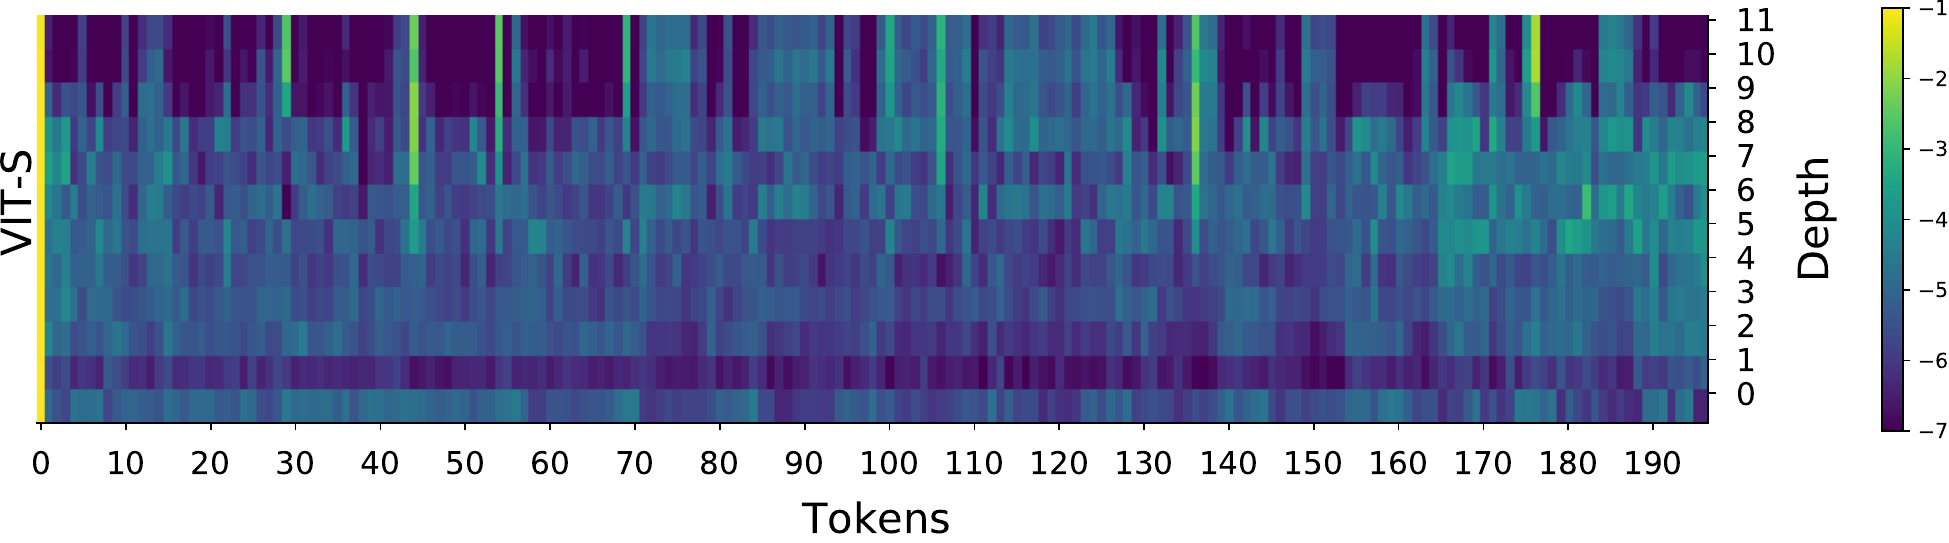} \\
        \includegraphics[width=.75\linewidth]{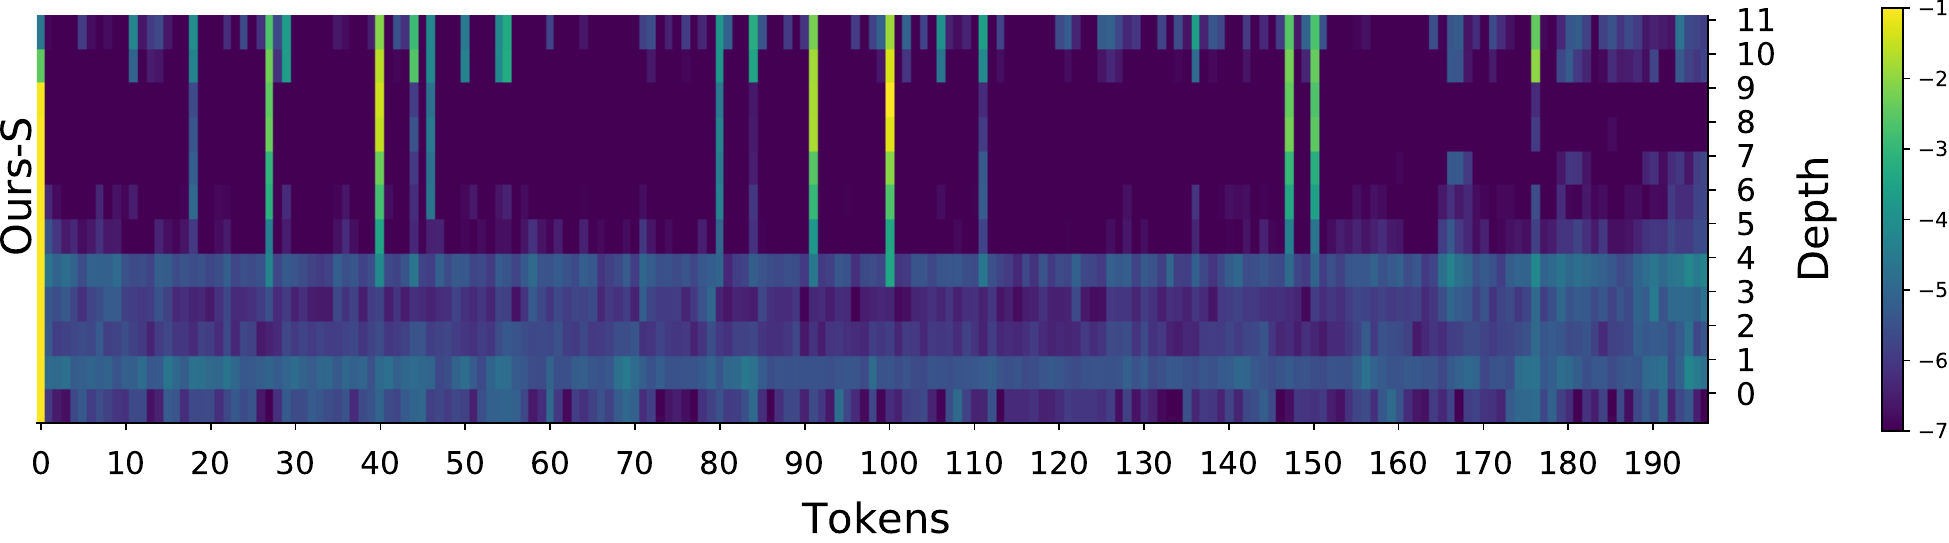} \\
    \end{tabular}
    \hrule
    \begin{tabular}{c}
        \includegraphics[width=.15\linewidth]{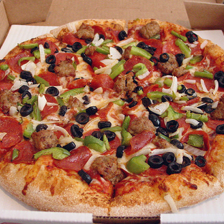}
    \end{tabular} %
    \begin{tabular}{c}
        \includegraphics[width=.75\linewidth]{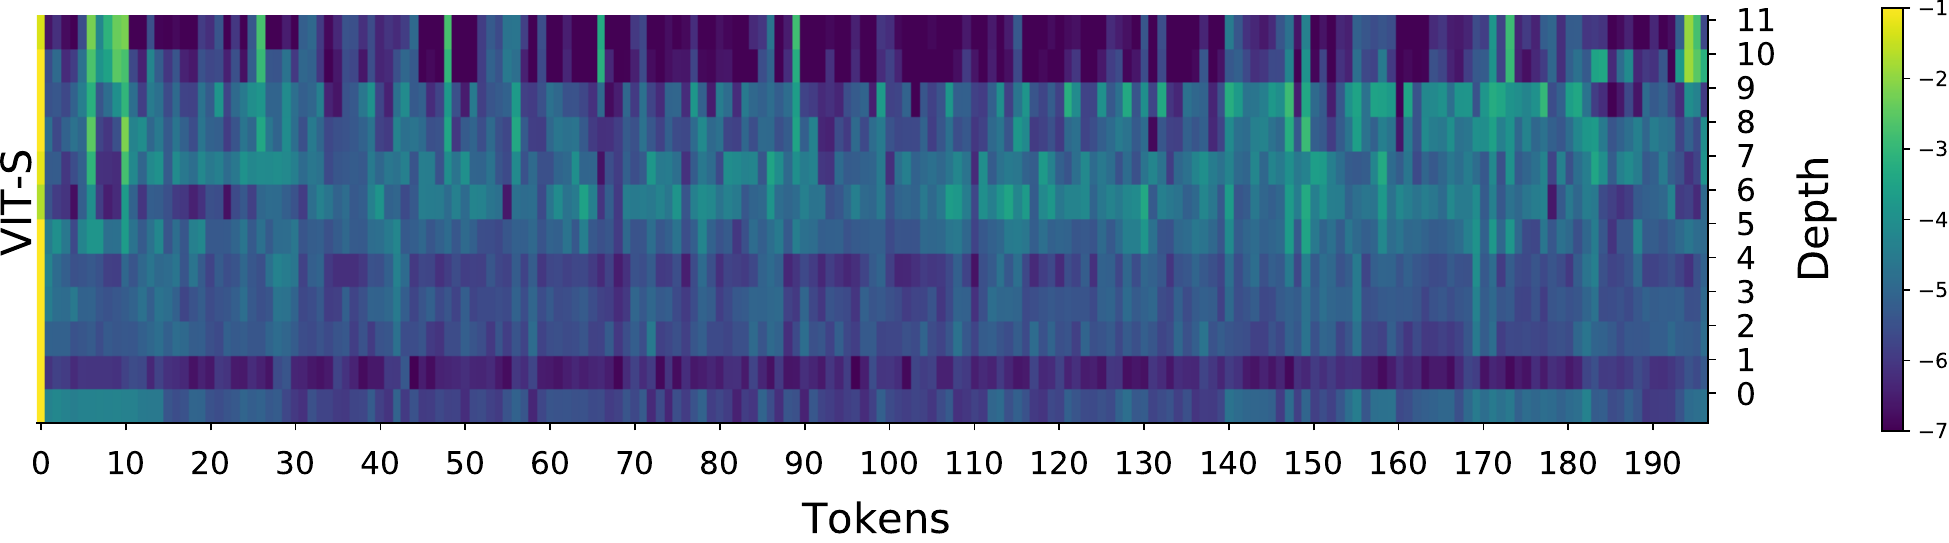} \\
        \includegraphics[width=.75\linewidth]{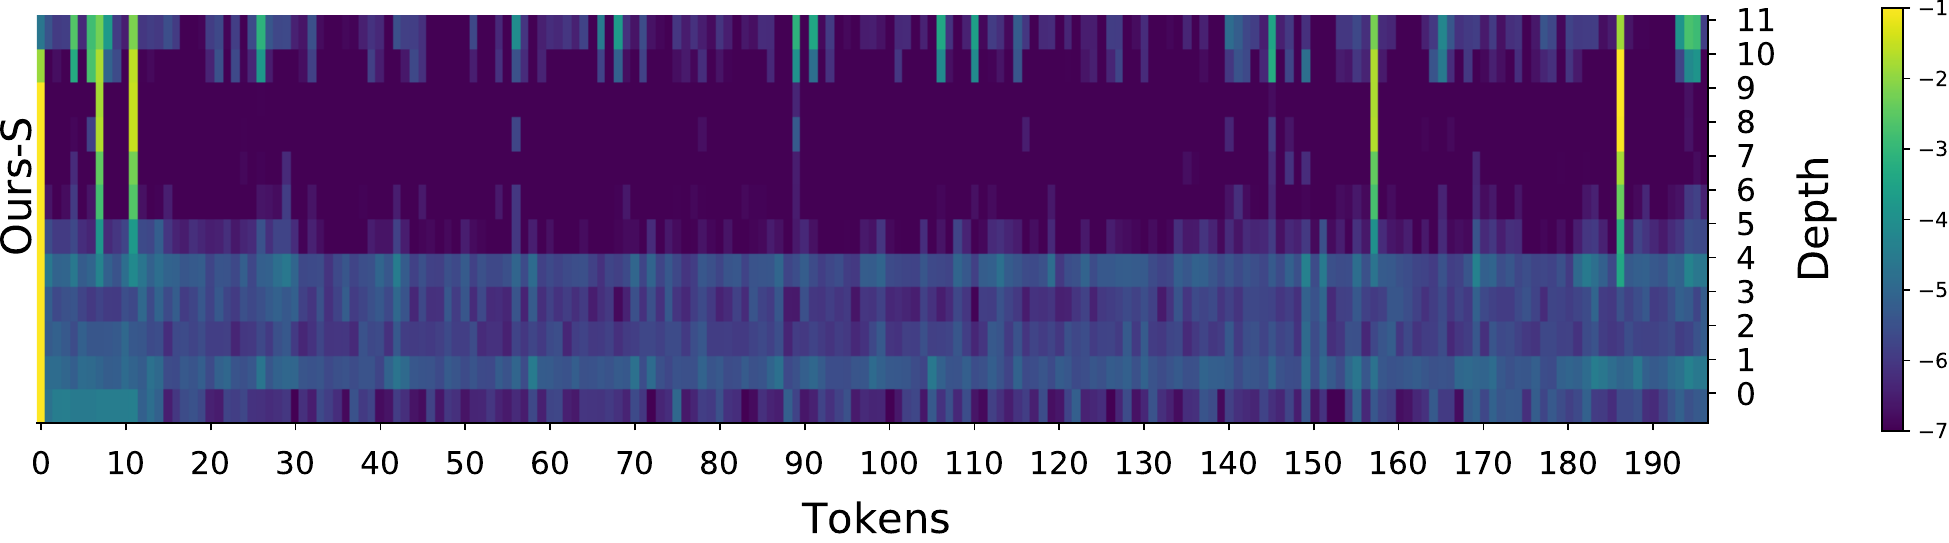} \\
    \end{tabular}
    \hrule
    \begin{tabular}{c}
        \includegraphics[width=.15\linewidth]{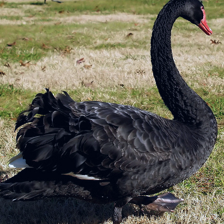}
    \end{tabular} %
    \begin{tabular}{c}
        \includegraphics[width=.75\linewidth]{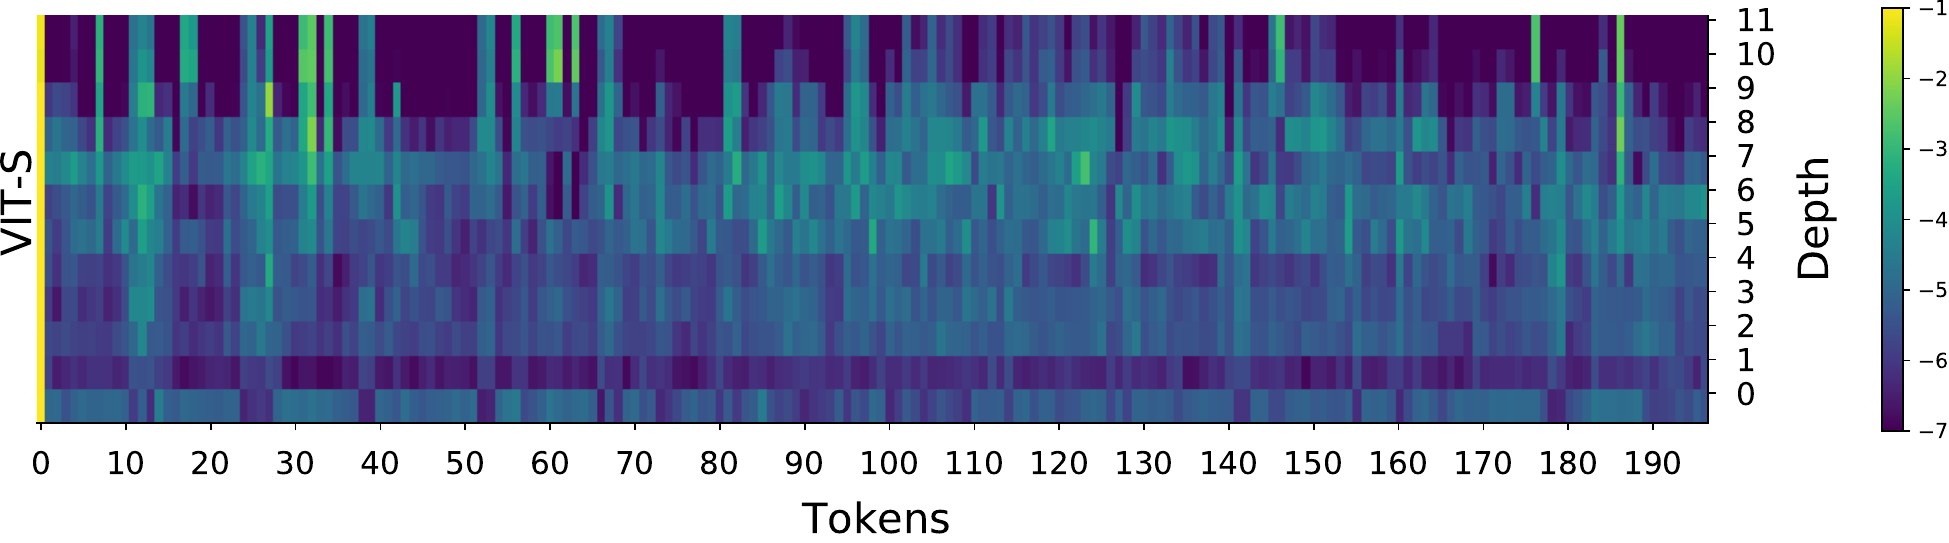} \\
        \includegraphics[width=.75\linewidth]{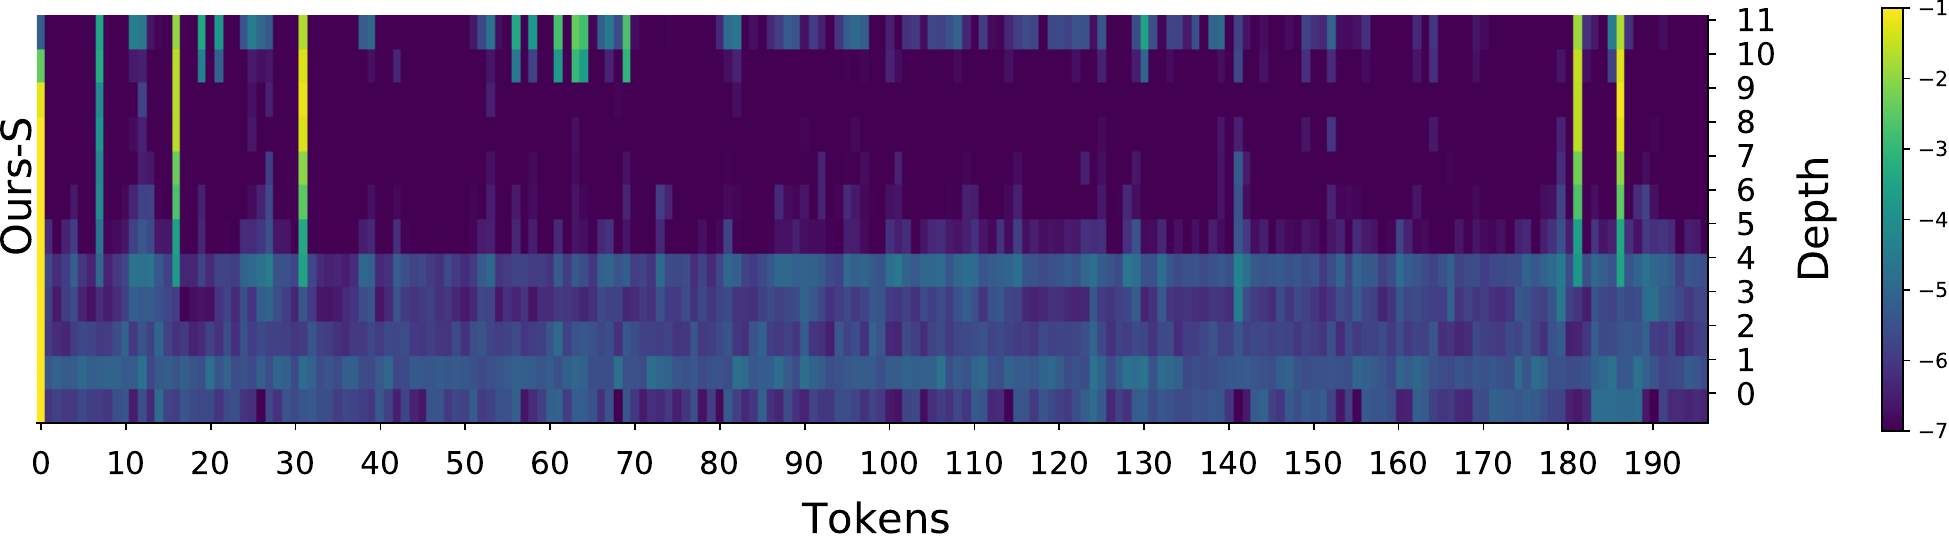} \\
    \end{tabular}
    
    \caption{\textbf{Visualization of attention corresponding with the class token.} $x$-axis and $y$-axis represent tokens and depth. We denote ViT-S with $\gs$ as Ours-S.
    In ViT-S and Ours-S, the number of tokens and depth are 197 and 12, respectively; thus, the attention map is $12 \times 197$. We apply the element-wise log operation to attention for visualization.}
    \label{fig:attn_vis}
\end{figure}
